# Supplementary material for: A Systematic Assessment of Syntactic Generalization in Neural Language Models
Source: arXiv:2005.03692 source file (2020-05-23)
Supplement: Supplementary file 1 [file correlation_appendix.tex]

%
% File acl2020.tex
%
%% Based on the style files for ACL 2020, which were
%% Based on the style files for ACL 2018, NAACL 2018/19, which were
%% Based on the style files for ACL-2015, with some improvements
%%  taken from the NAACL-2016 style
%% Based on the style files for ACL-2014, which were, in turn,
%% based on ACL-2013, ACL-2012, ACL-2011, ACL-2010, ACL-IJCNLP-2009,
%% EACL-2009, IJCNLP-2008...
%% Based on the style files for EACL 2006 by 
%%e.agirre@ehu.es or Sergi.Balari@uab.es
%% and that of ACL 08 by Joakim Nivre and Noah Smith

% \documentclass[11pt,a4paper]{article}
% \usepackage[hyperref]{acl2020}
% \usepackage{times}
% \usepackage{latexsym}
% \usepackage{booktabs}
% \usepackage{graphicx}
% \renewcommand{\UrlFont}{\ttfamily\small}
% \usepackage{microtype}
% \usepackage{amsmath}
% \usepackage{linguex-mod}
% \renewcommand{\firstrefdash}{}

% \aclfinalcopy
% \begin{document}

% \section*{Appendix B: Circuit--circuit correlations}
% \label{sec:circuit-correlations}

\begin{figure*}[ht]
    \begin{minipage}{\textwidth}
    \centering
    \includegraphics[width=1.2\textwidth]{figs/all-correlations.pdf}
    \caption{Circuit-circuit correlations.}
    \label{fig:all-circuit-correlations}
    \end{minipage}
\end{figure*}

In this appendix, we present results from analyzing the circuit-to-circuit correlation between the six syntactic circuits presented in the main body of this paper (Figure \ref{fig:all-circuit-correlations}). Each plot tracks the relationship between every trained model's average performance on two different circuits. Each point on a plot thus corresponds to a single model type, trained on a particular corpus, with a particular random seed. $N$-gram results are not included in the correlations.

Starting with the strongest correlations, we find that SG score on Agreement is positively correlated with all other circuits, except long-distance dependencies. The Agreement circuit consists exclusively of subject/verb number agreement dependencies. Given the abundance of subject/verb number agreement in English, success on this circuit may due to models' ability to track basic syntactic contingencies in the training data.

We find a significant positive correlation between Gross Syntactic State and Garden-Path Effects. Both of these circuits measure models' ability to use lexical, or low-level cues such as the presence of a comma, to drive expectations about larger upcoming syntactic chunks. The tight correlation between SG score on these two circuits may track models' general ability to track larger syntactic units that correspond to phrase-level chunks.

Turning to the extant but weaker correlations: We find a slight positive correlation between Long-Distance Dependencies and Garden Path effects. This may be due to the Cleft test suites in the Long-Distance Dependency circuit, which measures phenomena similar to the Garden-Path suites: models' expectation for VP and NP chunks following upstream conditioning tokens. We find a significant positive correlation between Licensing and Center Embedding, however this may be due to the presence of two outliers---both model$\times$training-data combinations that perform exceptionally well on both tests. We also find a slight correlation between Garden-Path and Center Embedding test suites.

%\bibliography{acl2020,rpl-journals-long,rpl}
% bibexport -o additional_references.bib
% test_suites_appendix_wrapper.aux
%\bibliography{acl2020}
%\bibliographystyle{acl_natbib}

% \end{document}
