# Supplementary material for: A Systematic Assessment of Syntactic Generalization in Neural Language Models
Source: arXiv:2005.03692 source file (2020-05-23)
Supplement: Supplementary file 2 [file test_suites_appendix_wrapper.tex]

%
% File acl2020.tex
%
%% Based on the style files for ACL 2020, which were
%% Based on the style files for ACL 2018, NAACL 2018/19, which were
%% Based on the style files for ACL-2015, with some improvements
%%  taken from the NAACL-2016 style
%% Based on the style files for ACL-2014, which were, in turn,
%% based on ACL-2013, ACL-2012, ACL-2011, ACL-2010, ACL-IJCNLP-2009,
%% EACL-2009, IJCNLP-2008...
%% Based on the style files for EACL 2006 by 
%%e.agirre@ehu.es or Sergi.Balari@uab.es
%% and that of ACL 08 by Joakim Nivre and Noah Smith

\documentclass[11pt,a4paper]{article}
\usepackage[hyperref]{acl2020}
\usepackage{times}
\usepackage{latexsym}
\usepackage{booktabs}

% This is not strictly necessary, and may be commented out,
% but it will improve the layout of the manuscript,
% and will typically save some space.
\usepackage{microtype}

\aclfinalcopy % Uncomment this line for the final submission
%\def\aclpaperid{***} %  Enter the acl Paper ID here

%\setlength\titlebox{5cm}
% You can expand the titlebox if you need extra space
% to show all the authors. Please do not make the titlebox
% smaller than 5cm (the original size); we will check this
% in the camera-ready version and ask you to change it back.

\newcommand{\textcite}[1]{\citet{#1}}

\usepackage{amsmath}
\usepackage{linguex-mod}

\title{Scaling up targeted syntactic evaluation of neural language models}

\author{First Author \\
  Affiliation / Address line 1 \\
  Affiliation / Address line 2 \\
  Affiliation / Address line 3 \\
  \texttt{email@domain} \\\And
  Second Author \\
  Affiliation / Address line 1 \\
  Affiliation / Address line 2 \\
  Affiliation / Address line 3 \\
  \texttt{email@domain} \\}

\date{}

\begin{document}
%these have to occur after \begin{document}
\setlength{\Extopsep}{.25\baselineskip}
\setlength{\Exlabelsep}{0.25cm} 
\setlength{\Exindent}{0cm} 
\setlength{\SubExleftmargin}{-0.55cm}

\input{test_suites_appendix}

%\bibliography{acl2020,rpl-journals-long,rpl}
% bibexport -o additional_references.bib
% test_suites_appendix_wrapper.aux
\bibliography{acl2020}
\bibliographystyle{acl_natbib}

\end{document}
